# Supplementary material for: Estimating the Adversarial Robustness of Attributions in Text with Transformers
Source: arXiv:2212.09155 source file (2022-12-18)
Supplement: Supplementary file 2 [file appendix_plots.tex]

\setlength{\plotwidth}{0.295\textwidth}%
\setlength{\plotheight}{0.23\textwidth}%
\addtolength{\tabcolsep}{-12pt}  % Default is 6pt
\addtolength{\rowsepoffset}{-5pt} % Default is 0pt
% [inline block 0: 1 envs, 51928 chars -> data_tex | \begin{longtable}[c]{cccc}     % First page head...]


\addtolength{\tabcolsep}{12pt}  % Default is 6pt 
\addtolength{\rowsepoffset}{5pt} % Default is 0pt
